# Supplementary material for: Autobahn: Automorphism-based Graph Neural Nets
Source: arXiv:2103.01710 source file (2022-02-03)
Supplement: Supplementary file 2 [file supplement2.pdf]

# Supplementary Information for Autobahn: Automorphism-based Graph Neural Nets

## 1 Activations as functions on a group

In the Autobahn formalism, we make extensive use of the fact that the activations of a group-equivariant neural network can be treated as functions on the same group. This formalism is covered in detail in Sections 3 and 4 of (Kondor & Trivedi, 2018), here we give a brief review for the unfamiliar reader.

Consider a space  $\mathcal{X}$  acted on by a group  $G$ : at every point  $x$  in  $\mathcal{X}$ , we can apply a group element  $g \in G$ , which maps  $x$  to another point in  $\mathcal{X}$ . The action of the group on  $\mathcal{X}$  induces an action on functions of  $\mathcal{X}$ . For any function  $f : \mathcal{X} \rightarrow \mathbb{C}$ , the group  $G$  has an induced group action

$$g(f)(x) = f(g(x)). \quad (1)$$

The inputs to group-equivariant neural networks are precisely functions on such spaces. For instance, for standard convolutional layers acting on images, each point on the space is a single pixel and the group of translation moves between pixels. The RGB value of each pixel is a vector-valued function of  $\mathcal{X}$ . Representations internal to the network, however, are not limited to being functions on  $\mathcal{X}$ . For instance, consider a neural network that is given a list of objects and attempts to learn an adjacency matrix. Both the list of objects and the adjacency matrix transform under permutation. Whereas each “point” in a list of objects corresponds to a single object, each “point” in the adjacency matrix corresponds to a pair of objects. While both the input and the output of the network transform according to permutation, they live on different spaces.

Fortunately, the complexity of dealing with a myriad of spaces can be avoided by mapping functions from their individual spaces to functions on  $G$ . For simplicity, we will assume that  $G$  is transitive on  $\mathcal{X}$ : for all  $x, y \in \mathcal{X}$ , there exists a group element  $g$  such that  $g(x) = y$ . (If the  $G$  is not transitive, we simply apply this procedure on every orbit of  $G$  and concatenate the results.) The construction proceeds as follows. We arbitrarily choose an initial point  $x_0$  in  $\mathcal{X}$  to act as the origin. Then, we construct the function

$$f_G(g) = f(g(x_0)). \quad (2)$$

In Figure 1, we depict this procedure, mapping the adjacency matrix for a graph with size 6 vertices to the  $S_6$ , the group of all permutations of six elements.

## 2 Proof of Equivariance for Autobahn

Here, we prove that the Autobahn architecture obeys permutation equivariance. For Autobahn, neural network inputs and activations are functions on subgroups acting on a reference domain, and global permutation of inputs can induce group operations in the associated subgroups.

To prove equivariance, we must first describe the transformation of Autobahn activations under global permutation. From Subsection 4.2, we recall that narrowing is the pseudoinverse of promotion. This implies that between every step in Autobahn, we can promote the activation of any neuron to  $\mathbb{S}_n$  and then immediately narrow it back to the neuron’s reference domain without changing the network. This allows us to rewrite the steps for an Autobahn neuron  $n_j^\ell$  as follows.

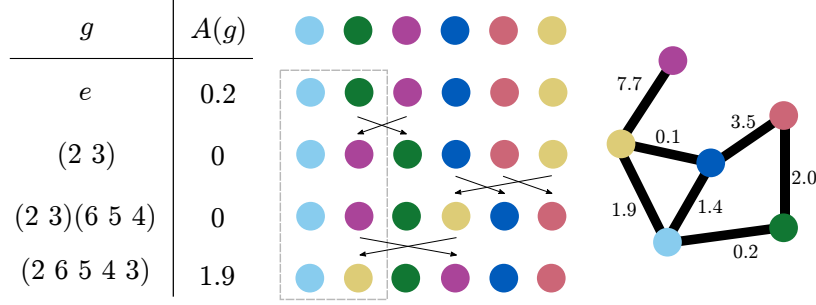

Figure 1: Example showing how function on the symmetric group can be constructed from neural network activations on the edges of a graph. We list the vertices in arbitrary order. We then construct the function as follows. For every permutation, we apply the permutation and look at two arbitrarily chosen vertices (here we have chosen the first two). If these vertices form an edge, the function takes the edge activation as its value. Otherwise, the function takes a value of zero.

T1.1 Narrow every activation  $f_{s_z}^{\ell-1}$  from  $S_n$  to  $(a_1^z, \dots, a_{m_z}^z)$ .

T1.2 Further narrow the incoming activation  $f_{s_z}^{\ell-1}$  to the corresponding intersection to get  $f_{s_z}^{\ell-1} \downarrow_{(b_1^z \dots b_{k_z}^z)}$ .

T1.3 Promote each  $f_{s_z}^{\ell-1} \downarrow_{(b_1^z \dots b_{k_z}^z)}$  to  $S_n$ .

T2.1 Narrow the results back to  $(b_1^z \dots b_{k_z}^z)$ .

T2.2 Promote each of these to  $(a_1, \dots, a_m)$ :

$$\tilde{f}_z = f_{s_z}^{\ell-1} \downarrow_{(b_1^z \dots b_{k_z}^z)} \uparrow^{(a_1 \dots a_m)}.$$

T2.3 Promote  $\tilde{f}_z$  to  $S_n$ .

T3.1 Narrow back down to  $(a_1, \dots, a_m)$ .

T3.2 Apply a symmetric polynomial  $S$  to  $\tilde{f}_1, \dots, \tilde{f}_p$ :

$$\hat{f} = S(\tilde{f}_1, \dots, \tilde{f}_p).$$

T3.3 Promote  $\hat{f}$  to  $S_n$ .

T4.1 Narrow back down to  $(a_1, \dots, a_m)$ .

T4.2 Apply one or more (learnable) equivariant linear transformations  $\psi_j$ , each of which is followed by a fixed pointwise nonlinearity  $\xi$ , to get the final output of the neuron.

$$f_j^\ell = \xi(\psi_j(\hat{f})).$$

T4.3 Promote every  $f_j^\ell$  to  $S_n$ .

Here, we have rewritten Autobahn so that T1-T4 all map functions on  $S_n$  to functions on  $S_n$ . To show equivariance, we will show that each of these steps is equivariant to permutation in  $S_n$  and independent of the ordering within the reference domain.

## 2.1 Action of global permutations and narrowing and promotion

To relate global permutations with actions on individual reference domains, it will be helpful to define two operations that relate permutations on smaller subsets to permutations on a larger space. Let  $\mu$  be a permutation in  $S_m$ . We define a permutation in  $S_{n>m}$ , which we denote as  $\dot{\mu}$ , as the permutation that applies  $\mu$  to the first  $m$  indices and leaves the rest untouched.

$$\begin{aligned} \dot{\mu}(p) = q &\iff \mu(p) = q && \forall p, q \in \{1, \dots, m\} \\ \dot{\mu}(p) = p &&& \forall p \in \{m+1, \dots, n\}. \end{aligned} \quad (3)$$

Similarly, we define  $\dot{\mu}$  to be the permutation that applies  $\mu$  to the last  $m$  and leaves the first  $n - m$  indices untouched.

$$\begin{aligned} \dot{\mu}(p) = q &\iff \mu(p - n + m) = q - n + m & \forall p, q \in \{n - m + 1, \dots, n\} \\ \dot{\mu}(p) = p & & \forall p \in \{1, \dots, n - m\} \end{aligned} \quad (4)$$

Now, we consider the ordered subset  $(i_1, \dots, i_m)$ . If  $a$  is a permutation sends  $(1, \dots, m)$  to  $\{i_1, \dots, i_m\}$ , it can be written as

$$a = t\dot{u}\dot{v} \quad (5)$$

where  $u \in \mathbb{S}_m$ ,  $v \in \mathbb{S}_{n-m}$ , and  $t$  is an arbitrarily chosen permutation that sends  $(1, \dots, m)$  to  $(i_1, \dots, i_m)$ . For a given choice of  $t$ , this decomposition is unique. Narrowed functions can consequently be written as

$$f\downarrow_{(i_1, \dots, i_m)}(u\downarrow_{(i_1, \dots, i_m)}) = \sum_v f(t\dot{u}\dot{v}) \quad (6)$$

and promoted functions can be written as

$$g\uparrow^{(i_1, \dots, i_m)}(a) = \begin{cases} g(u) & \text{if } \exists u \in \mathbb{S}_m, v \in \mathbb{S}_{n-m} \text{ s.t. } a = t\dot{u}\dot{v} \\ 0 & \text{otherwise.} \end{cases} \quad (7)$$

We now consider how a permutation  $\sigma$  affects narrowing and promotion. If  $a$  sends  $(1, \dots, m)$  to  $\{i_1, \dots, i_m\}$ , then  $\sigma a$  sends  $(1, \dots, m)$  to  $\{\sigma(i_1), \dots, \sigma(i_m)\}$ . However, since the ordering in each reference domain is chosen arbitrarily, the reference for the corresponding neuron in the permuted network is, in general, *not*  $(\sigma(i_1), \dots, \sigma(i_m))$ . Let  $\tau$  be a permutation that sends  $(1, \dots, m)$  to the reference domain of the neuron in the permuted network. In analogy to (5), we can define  $\mu \in \mathbb{S}_m$  and  $\nu \in \mathbb{S}_{n-m}$  su that

$$\alpha = \tau\dot{\mu}\dot{\nu} \quad (8)$$

for any  $\alpha \in \mathbb{S}_n$  that sends  $(1, \dots, m)$  to the set  $\{\sigma(i_1), \dots, \sigma(i_m)\}$ . This suggests that there must exist  $s \in \mathbb{S}_m$ ,  $w \in \mathbb{S}_{n-m}$  such that

$$\tau\dot{s}\dot{w} = \sigma t. \quad (9)$$

Consequently, we have

$$\mathbb{T}_\sigma f(\alpha) = \mathbb{T}_\sigma f(\sigma t \dot{s}^{-1} \dot{w}^{-1} \dot{\mu} \dot{\nu}) = f(t(\dot{s}^{-1} \dot{\mu})(\dot{w}^{-1} \dot{\nu})) \quad (10)$$

allowing us to identify

$$u = s^{-1}\mu, \quad v = w^{-1}\nu. \quad (11)$$

With this terminology established, we can determine how narrowed and promoted functions transform when applying a global permutation to the network. Narrowed functions transform as

$$\left( (\mathbb{T}_\sigma f)\downarrow_{(\sigma(i_{s^{-1}(1)}), \dots, \sigma(i_{s^{-1}(k)}))} \right) (\mu) = \sum_\nu \mathbb{T}_\sigma f(\tau\dot{\mu}\dot{\nu}) \quad (12)$$

$$= \sum_\nu f(t\dot{s}^{-1}\dot{\mu}\dot{\nu}) \quad (13)$$

$$= f\downarrow_{(i_1, \dots, i_k)}(s^{-1}\mu) \quad (14)$$

$$= \mathbb{T}_s \left( f\downarrow_{(i_1, \dots, i_k)} \right) (\mu) \quad (15)$$

and promoted functions transform as

$$g\uparrow^{(\sigma(i_{s^{-1}(1)}), \dots, \sigma(i_{s^{-1}(k)}))}(\alpha) = \begin{cases} g(\mu) & \text{if } \exists \mu \in \mathbb{S}_k, \nu \in \mathbb{S}_{m-k} \text{ s.t. } \alpha = \tau\dot{\mu}\dot{\nu} \\ 0 & \text{otherwise.} \end{cases} \quad (16)$$

$$= \begin{cases} g(su) & \text{if } \exists \mu \in \mathbb{S}_k, \nu \in \mathbb{S}_{m-k} \text{ s.t. } \alpha = \sigma t \dot{u} \dot{v} \\ 0 & \text{otherwise.} \end{cases} \quad (17)$$

$$\implies \mathbb{T}_s g\uparrow^{(\sigma(i_{s^{-1}(1)}), \dots, \sigma(i_{s^{-1}(k)}))} = (\mathbb{T}_\sigma g)\uparrow^{(i_1, \dots, i_k)} \quad (18)$$

$$\begin{array}{ccccc}
(2, 4, 3, \dots) & \xleftarrow[p^{-1}]{\dot{p}} & (1, 2, 3, 4, 5, \dots) & \xleftarrow[t^{-1}]{\dot{t}} & (\dots, 5, 3, \dots, 2, 1, \dots, 4, \dots) \\
\psi^{-1} \dot{\chi}^{-1} \uparrow \downarrow \psi \dot{\chi} & & s^{-1} \dot{w}^{-1} \uparrow \downarrow s \dot{w} & & \sigma^{-1} \uparrow \downarrow \sigma \\
(4, 2, 3, \dots) & \xleftarrow[\pi^{-1}]{\pi} & (5, 4, 1, 3, 2, \dots) & \xleftarrow[\tau^{-1}]{\tau} & (\dots, 4, 3, \dots, 5, \dots, 2, 4, 1)
\end{array}$$

Figure 2: Commutative diagram depicting the permutations involved in T1 and T2. For concreteness, we have set  $k = 3$  and  $m = 5$ . The reference domain corresponding to  $(i_1, \dots, i_m)$  contains of vertices 1 through 5, and the reference domain corresponding to  $(j_1, \dots, j_k)$  consists of vertices 4, 2, and 3.

## 2.2 Proof of equivariance for individual sublayers

We now prove that each of the individual sublayers T1-T4 obey equivariance.

### 2.2.1 T1 is equivariant

Since we are applying narrowing twice, we must deal with two reference domains:  $(i_1 \dots i_m)$  and the reference domain formed by a subset,  $(j_1, \dots, j_k)$ . Throughout this section, we will extend the notation introduced in (3) and (4) to maps from  $\mathbb{S}_k$  to  $\mathbb{S}_m$  or  $\mathbb{S}_k$  to  $\mathbb{S}_n$  as necessary, and trust that the precise domain and ranges of the maps will be clear from context.

In analogy with (5) and (8), we can write any permutation that sends  $(1, \dots, k)$  to  $\{j_1, \dots, j_k\}$  as

$$b = p\dot{q}\dot{r} \quad (19)$$

where  $q \in \mathbb{S}_k$ ,  $r \in \mathbb{S}_{m-k}$ , and  $p \in \mathbb{S}_m$  is an arbitrarily chosen permutation that sends  $(1, \dots, k)$  to  $(j_1, \dots, j_k)$ . Similarly, we define

$$\beta = \pi\dot{\phi}\dot{\rho} \quad (20)$$

for the analogous reference domain formed in the permuted net, and let  $\psi \in \mathbb{S}_k$  and  $\chi \in \mathbb{S}_{m-k}$  be permutations such that

$$\pi\dot{\psi}\dot{\chi} = ps. \quad (21)$$

The global permutation  $\sigma$  then transforms the reference domain  $(j_1, \dots, j_k)$  as follows

$$(j_i, \dots, j_k) \xrightarrow{\sigma} (s(j_{\psi^{-1}(1)}), \dots, s(j_{\psi^{-1}(k)})) \quad (22)$$

in the permuted network. To aid the reader, we have summarized the actions of the permutations on the various reference domains in Figure 2.

We now seek to prove equivariance:

$$\begin{aligned}
& \left( \left( (\mathbb{T}_\sigma f) \downarrow (\sigma(i_{s^{-1}(1)}), \dots, \sigma(i_{s^{-1}(m)})) \right) \downarrow (s(j_{\psi^{-1}(1)}), \dots, s(j_{\psi^{-1}(k)})) \right) \uparrow \left( \sigma(i_{j_{\psi^{-1}(1)}}), \dots, \sigma(i_{j_{\psi^{-1}(k)}}) \right) \\
& = \mathbb{T}_\sigma \left( \left( (f \downarrow (i_1, \dots, i_m)) \downarrow (j_1, \dots, j_k) \right) \uparrow (i_{j_1}, \dots, i_{j_k}) \right)
\end{aligned} \quad (23)$$

Repeatedly applying (15), we have

$$\begin{aligned}
& \left( \left( (\mathbb{T}_\sigma f) \downarrow (\sigma(i_{s^{-1}(1)}), \dots, \sigma(i_{s^{-1}(m)})) \right) \downarrow (s(j_{\psi^{-1}(1)}), \dots, s(j_{\psi^{-1}(k)})) \right) \uparrow \left( \sigma(i_{j_{\psi^{-1}(1)}}), \dots, \sigma(i_{j_{\psi^{-1}(k)}}) \right) \\
& = \left( \left( \mathbb{T}_s (f \downarrow (i_1, \dots, i_k)) \right) \downarrow (s(j_{\psi^{-1}(1)}), \dots, s(j_{\psi^{-1}(k)})) \right) \uparrow \left( \sigma(i_{j_{\psi^{-1}(1)}}), \dots, \sigma(i_{j_{\psi^{-1}(k)}}) \right)
\end{aligned} \quad (24)$$

$$= \left( \mathbb{T}_\psi \left( \left( (f \downarrow (i_1, \dots, i_k)) \downarrow (j_1, \dots, j_k) \right) \right) \uparrow \left( \sigma(i_{j_{\psi^{-1}(1)}}), \dots, \sigma(i_{j_{\psi^{-1}(k)}}) \right) \right) \quad (25)$$

$$= \mathbb{T}_\sigma \left( \left( (f \downarrow (i_1, \dots, i_k)) \downarrow (j_1, \dots, j_k) \right) \right) \uparrow \left( \sigma(i_{j_1}), \dots, \sigma(i_{j_k}) \right) \quad (26)$$

where the last line follows by the same argument as (18).

### 2.2.2 T2 is equivariant

We seek to prove that

$$\begin{aligned} & \left( \left( (\mathbb{T}_\sigma f) \downarrow_{(\sigma(i_{j_\psi-1(1)}), \dots, \sigma(i_{j_\psi-1(k)}))} \right) \uparrow^{(s(j_{\psi-1(1)}), \dots, s(j_{\psi-1(k)}))} \right) \uparrow^{(\sigma(i_{s-1(1)}), \dots, \sigma(i_{s-1(m)}))} \\ &= \mathbb{T}_\sigma \left( \left( (f \downarrow_{(i_{j_1}, \dots, i_{j_k})}) \uparrow^{(j_1, \dots, j_k)} \right) \uparrow^{(i_1, \dots, i_m)} \right) \end{aligned} \quad (27)$$

The proof proceeds similarly to the proof for T1. We have

$$\begin{aligned} & \left( \left( (\mathbb{T}_\sigma f) \downarrow_{(\sigma(i_{j_\psi-1(1)}), \dots, \sigma(i_{j_\psi-1(k)}))} \right) \uparrow^{(s(j_{\psi-1(1)}), \dots, s(j_{\psi-1(k)}))} \right) \uparrow^{(\sigma(i_{s-1(1)}), \dots, \sigma(i_{s-1(m)}))} \\ &= \left( \left( \mathbb{T}_\psi \left( f \downarrow_{(i_{j_1}, \dots, i_{j_k})} \right) \right) \uparrow^{(s(j_{\psi-1(1)}), \dots, s(j_{\psi-1(k)}))} \right) \uparrow^{(\sigma(i_{s-1(1)}), \dots, \sigma(i_{s-1(m)}))} \end{aligned} \quad (28)$$

$$= \left( \mathbb{T}_s \left( \left( f \downarrow_{(i_{j_1}, \dots, i_{j_k})} \right) \uparrow^{(j_1, \dots, j_k)} \right) \right) \uparrow^{(\sigma(i_{s-1(1)}), \dots, \sigma(i_{s-1(m)}))} \quad (29)$$

$$= \mathbb{T}_\sigma \left( \left( (f \downarrow_{(i_{j_1}, \dots, i_{j_k})}) \uparrow^{(j_1, \dots, j_k)} \right) \uparrow^{(i_1, \dots, i_m)} \right) \quad (30)$$

### 2.2.3 T3 is equivariant

To prove that applying a symmetric polynomial and applying convolution over a graph's automorphism group preserves equivariance, we require the following lemma.

**Lemma 1.** *Let  $A$  be an  $\mathbb{S}_m$  equivariant operator. Then,*

$$\left( A \left( (\mathbb{T}_\sigma f) \downarrow_{(\sigma(i_{s-1(1)}), \dots, \sigma(i_{s-1(k)}))} \right) \right) \uparrow^{(\sigma(i_{s-1(1)}), \dots, \sigma(i_{s-1(k)}))} = \mathbb{T}_\sigma f \left( \left( A \left( f \downarrow_{(i_1, \dots, i_k)} \right) \right) \uparrow^{(i_1, \dots, i_k)} \right) \quad (31)$$

*Proof.* Applying (15), the definition of equivariance, and (18) we have

$$\begin{aligned} & \left( A \left( (\mathbb{T}_\sigma f) \downarrow_{(\sigma(i_{s-1(1)}), \dots, \sigma(i_{s-1(k)}))} \right) \right) \uparrow^{(\sigma(i_{s-1(1)}), \dots, \sigma(i_{s-1(k)}))} \\ &= \left( A \left( \mathbb{T}_s \left( f \downarrow_{(i_1, \dots, i_m)} \right) \right) \right) \uparrow^{(\sigma(i_{s-1(1)}), \dots, \sigma(i_{s-1(k)}))} \\ &= \left( \mathbb{T}_s \left( A \left( f \downarrow_{(i_1, \dots, i_m)} \right) \right) \right) \uparrow^{(\sigma(i_{s-1(1)}), \dots, \sigma(i_{s-1(k)}))} \\ &= \mathbb{T}_\sigma f \left( \left( A \left( f \downarrow_{(i_1, \dots, i_k)} \right) \right) \uparrow^{(i_1, \dots, i_k)} \right) \end{aligned} \quad (32)$$

□

To prove equivariance of T3, it is therefore enough to prove that application of the symmetric polynomial is  $\mathbb{S}_m$ -equivariant. Indeed, permutation of the reference domain could permute the arbitrary order of the functions input to the polynomial. However, the output of the polynomial is invariant by definition, and it is well-known that the products are group-equivariant (Kondor et al., 2018). Consequently, the symmetric polynomials obey equivariance.

### 2.2.4 T4 is equivariant

Lemma 1 implies that it is enough for automorphism-based convolutions to be equivariant to permutations within the reference domain. Our automorphism-based convolutions can be written as

$$\mathbb{T}_b B \mathbb{T}_{b^{-1}} \quad (33)$$

where  $B$  is a convolution over the Automorphism group of the subgraph and  $b$  is an arbitrarily chosen permutation that sends the graph in a canonical position to it's current labeling. Upon applying a global permutation  $\sigma$ , the neuron in the permuted net must find a new permutation  $\beta$  to send the permuted graph into the correct position. Consequently, we seek to prove that

$$\mathbb{T}_\beta B \mathbb{T}_{\beta^{-1}} (\mathbb{T}_s f) = \mathbb{T}_s (\mathbb{T}_b B \mathbb{T}_{b^{-1}} f) \quad (34)$$

Since the choice of  $\beta$  and  $b$  is arbitrary, they can be related by an unknown permutation  $\gamma$  that corresponds to an automorphism on the subgraph.

$$\beta\gamma = sb\gamma^{-1} \quad (35)$$

(The similarity to (9) is not coincidental: the decomposition into a smaller reference domain corresponds to the automorphism group of a graph with two fully connected disjoint components.) Consequently, we have

$$\mathbb{T}_\beta B \mathbb{T}_{\beta^{-1}} \mathbb{T}_s f = \mathbb{T}_\beta B \mathbb{T}_\gamma \mathbb{T}_{b^{-1}} f \quad (36)$$

$$= \mathbb{T}_\beta \mathbb{T}_\gamma B \mathbb{T}_{b^{-1}} f \quad (37)$$

$$= \mathbb{T}_s \mathbb{T}_b B \mathbb{T}_{b^{-1}} f \quad (38)$$

completing the proof.

### 3 Writing GCN as an Autobahn Network

As an example to illustrate the connection between Autobahn networks and message passing networks, we construct an Autobahn that corresponds to a simple MPNN. The architecture, modulo slight modifications, is the same as the one described in (Kipf & Welling, 2017).

In the language of Autobahn, message-passing networks correspond to reference domains constructed from star graphs. To construct a graph convolutional network in the language of Autobahn, for each vertex  $v_i$  we construct a neuron  $\mathfrak{n}_i^\ell$  whose reference domains consist of all the vertices with directed edges that point to  $v_i$ . The initial activation for each neuron is set to be constant over permutations, with the constant value set to be the initial node feature. In each layer, a neuron  $\mathfrak{n}_i^\ell$  then performs the following operations. For simplicity, we have omitted normalizations by the degree of each node and are omitting the skip-connections in each neuron (corresponding to the diagonal term in the adjacency matrix). These can easily be incorporated in the architecture, e.g. in steps T1 and T3.

- T1. Narrow incoming activations to the corresponding intersections. By construction, this intersection is only nonzero if  $\mathfrak{n}_i^{\ell-1}$  and  $\mathfrak{n}_{s_z}^{\ell-1}$  correspond to adjacent neurons in the graph. The corresponding intersection is exactly the set  $\{v_i, v_{s_z}\}$ .
- T2. Promote to  $\mathfrak{R}_i^\ell$ . Each promoted function is constant on any permutation that sends the set  $\{v_i, v_{s_z}\}$  to itself, and is zero otherwise.
- T3. Aggregate the narrowed activations via summation.
- T4. Sum over all permutations in the reference domain. This corresponds to a convolution against the constant function. Finally, we apply a learned linear transformation over channels, followed by a fixed nonlinearity.

To see that this is the same as a GCN-like architecture, we observe that each promoted function corresponds to one neighboring vertex. Moreover, each promoted function comes from an intersection of the same size (a set of size 2). Consequently, each promoted function is represented in the same number of permutations, and the output of steps T1-T4 are equivalent to summing over the activation of each neighboring vertex.

### 4 Architecture, hyper-parameter and computational details

We provide some further details into the architecture, choice of hyper-parameters and training regime of our network.

| Modification              | Validation loss   |
|---------------------------|-------------------|
| Original                  | $0.124 \pm 0.001$ |
| No cycles                 | $0.175 \pm 0.004$ |
| Only maximum length paths | $0.167 \pm 0.001$ |

Table 1: Validation loss for modified architectures on the Zinc (subset) dataset.

| Dataset       | Channels | Dropout | Epochs | Warmup | Decay milestones |
|---------------|----------|---------|--------|--------|------------------|
| Zinc (subset) | 128      | 0.0     | 600    | 15     | 150, 300         |
| Zinc          | 128      | 0.0     | 150    | 5      | 40, 80           |
| MolPCBA       | 128      | 0.0     | 50     | 5      | 35               |
| MolHIV        | 128      | 0.5     | 60     | 15     | N/A              |
| MolMUV        | 64       | 0.0     | 30     | 5      | N/A              |

Table 2: Hyper-parameter and training schedules used on each dataset.

#### 4.1 Architecture details

We model our block specific (i.e. cycle / path) convolutions after standard residual convolutional networks (He et al., 2016) with ReLU activations. We refer the reader to our pytorch implementation for details of the implementation.

We perform a simple ablation study of the main components of the model on the Zinc-subset problem. In particular, we study the impact of omitting: i) the cycle-based convolutions and ii) the paths shorter than the maximum length considered. Validation loss<sup>1</sup> results are reported in table 1.

#### 4.2 Hyper-parameter details

Our hyper-parameters were chosen based on a combination of chemical intuition and cursory data-based selection, with some consideration towards computational cost. As our architecture specification is quite general, the number of hyper-parameters is potentially large. In practice, we have restricted ourselves to tuning three parameters: a global network width parameter (which controls the number of channels in all convolutional and linear layers), a dropout parameter (which controls whether dropout is used and the amount of dropout), and the training schedule. The values used are specified in table 2. The training schedule is set with a base learning rate of 0.0003 at batch size 128 (and scaled linearly with batch size). The learning rate is increased linearly from zero to the base rate during the specified number of warmup epochs, and is then piecewise-constant, with the value decaying by a factor of 10 after each milestone.

The lengths of the paths and cycles considered in the model are also hyper-parameters of the model. We used the same values (cycles of lengths 5 and 6, and paths of lengths 3 to 6 inclusive) in all of our models. We note that in molecular graphs, cycles of lengths other than 5 and 6 are exceedingly rare (e.g. in the Zinc dataset, cycles of lengths different from 5 or 6 appear in about 1% of the molecules). We evaluate different possibilities for the maximum length of paths to be considered in table 3, we observe that in general, both computational time and prediction performance increase with larger path lengths.

#### 4.3 Computational details

In a message passing graph neural network, computational time is typically proportional to the number of edges present in the graph. On the other hand, our Autobahn network scales with the number of paths and

<sup>1</sup>Note that for this particular dataset, validation losses tend to be higher than test losses, which is also observed in some other architectures such as HIMP.

| Path length | Validation Loss   | Training Time |
|-------------|-------------------|---------------|
| 4           | $0.140 \pm 0.000$ | 3 h15 min     |
| 5           | $0.135 \pm 0.000$ | 4 h50 min     |
| 6           | $0.124 \pm 0.000$ | 6 h50 min     |
| 7           | $0.121 \pm 0.001$ | 9 h30 min     |

Table 3: Performance and training time of model on Zinc (subset) as a function of maximum path length considered.

cycles present in the graph. An immediate concern may be that the number of such structures could be combinatorially large in the size of the graph. In table 4, we show that, due to their tree-like structure, molecular graphs do not display such combinatorial explosion of number of sub-structures in practice.

The computational cost of our model scales roughly linearly with the total number of substructures under consideration. In practice, for molecular graphs, selecting only paths of short lengths and cycles, we expect the computational cost to be on the same order of magnitude as standard graph neural networks. We report the total amount of time (in GPU-hours) required for training each of our model in table 5. The training was performed on Nvidia V100 GPUs, and mixed-precision computation was used for all models except MolHIV where some gradient stability issue were encountered. The two largest datasets (Zinc and MolPCBA) were trained on four GPUs, whereas the remaining datasets were trained on a single GPU.

| Dataset | Nodes | Edges | Paths |      |      |      |      |       | Cycles |      |
|---------|-------|-------|-------|------|------|------|------|-------|--------|------|
|         |       |       | 3     | 4    | 5    | 6    | 7    | 8     | 5      | 6    |
| Zinc    | 23.1  | 49.8  | 34.6  | 43.9 | 55.0 | 64.4 | 65.8 | 70.2  | 0.56   | 1.70 |
| MolPCBA | 26.0  | 56.3  | 39.3  | 51.0 | 65.2 | 79.5 | 84.2 | 93.1  | 0.50   | 2.23 |
| MolHIV  | 25.5  | 54.9  | 39.2  | 52.1 | 68.9 | 87.2 | 97.2 | 111.5 | 0.34   | 2.01 |
| MolMUV  | 24.2  | 52.5  | 36.5  | 47.6 | 61.1 | 73.4 | 77.2 | 84.6  | 0.63   | 2.02 |

Table 4: Average count of structures in various datasets.

| Dataset       | Samples | Samples / s / GPU | Training time (GPU-hours) |
|---------------|---------|-------------------|---------------------------|
| Zinc (subset) | 6.0M    | 280               | 6.8 h                     |
| Zinc          | 33.0M   | 215               | 42.7 h                    |
| MolPCBA       | 21.9M   | 171               | 35.5 h                    |
| MolHIV        | 2.5M    | 114               | 6.1 h                     |
| MolMUV        | 2.8M    | 222               | 3.5 h                     |

Table 5: Computational cost of training provided models. Samples denotes total number of gradients computed (i.e. number of epochs times number of observations in dataset).

## References

- He, K., Zhang, X., Ren, S., and Sun, J. Deep residual learning for image recognition. In *Proceedings of the IEEE conference on computer vision and pattern recognition*, pp. 770–778, 2016.
- Kipf, T. N. and Welling, M. Semi-supervised classification with graph convolutional networks. In *International Conference on Learning Representations (ICLR)*, 2017.



Kondor, R. and Trivedi, S. On the generalization of equivariance and convolution in neural networks to the action of compact groups. In *Proceedings of International Conference on Machine Learning (ICML)*, 2018.

Kondor, R., Lin, Z., and Trivedi, S. Clebsch–Gordan nets: a fully Fourier space spherical convolutional neural network. *ArXiv e-prints*, 1806.09231, June 2018.
